# Supplementary material for: Unsupervised Domain Adaptation from Axial to Short-Axis Multi-Slice Cardiac MR Images by Incorporating Pretrained Task Networks
Source: arXiv:2101.07653 source file (2021-01-20)
Supplement: Supplementary file 2 [file arxiv_supplement.tex]

\title{Supplemental Material to: \\ Unsupervised Domain Adaptation from Axial to \\ Short-Axis Multi-Slice Cardiac MR Images by \\ Incorporating Pretrained Task Networks}
\author{Sven Koehler et al.}

\maketitle

\begin{figure}[t]

\begin{minipage}{1\linewidth}
\begin{figure}
\centering
    \includegraphics[height=0.3\textheight]{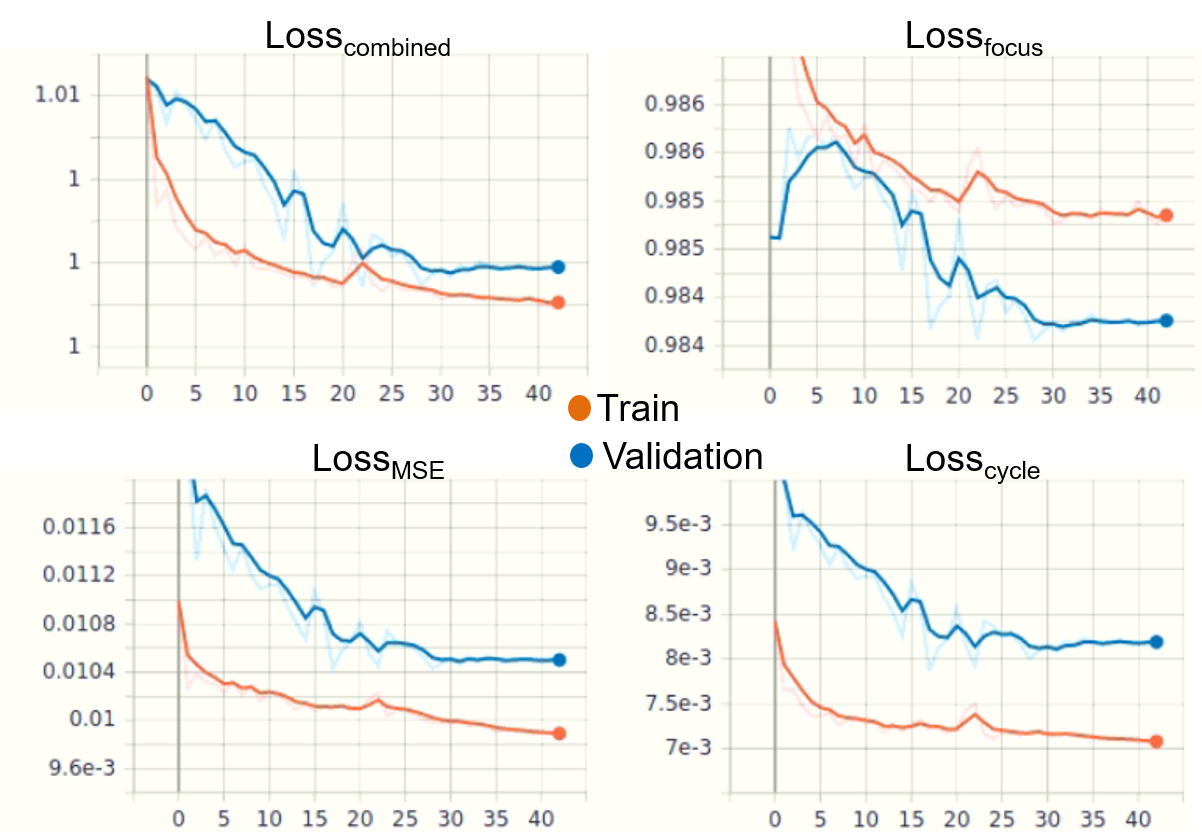}
  \caption{Training- and validation loss per epoch for each of the loss functions for one random fold of the full pipeline (with all extensions). Note the different scales on the $y$-axis, which led to $\alpha_{1}= 1.0$, and $\alpha_{2}= 0.1$ in $Loss = \alpha_{1} Loss_{Cycle} + \alpha_{2} Loss_{Focus}$.}
  \label{fig:tmilearning}
\end{figure}
\end{minipage}

\begin{minipage}{1\linewidth}
\begin{figure}
    \centering
  \includegraphics[height=0.1\textheight]{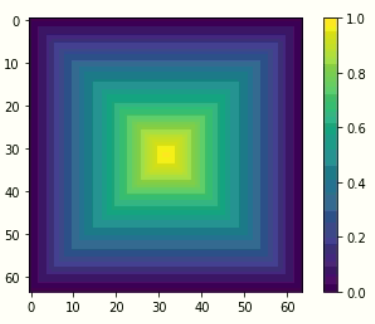}
  \caption{Soft linear in-plane weighting map $W$ in Eqn. (13), which guided the loss to focus on the center instead of border areas.}
  \label{fig:inplaneweighting}
\end{figure}

\end{minipage}

\begin{minipage}{1\linewidth}
\centering
  \includegraphics[height=0.25\textheight]{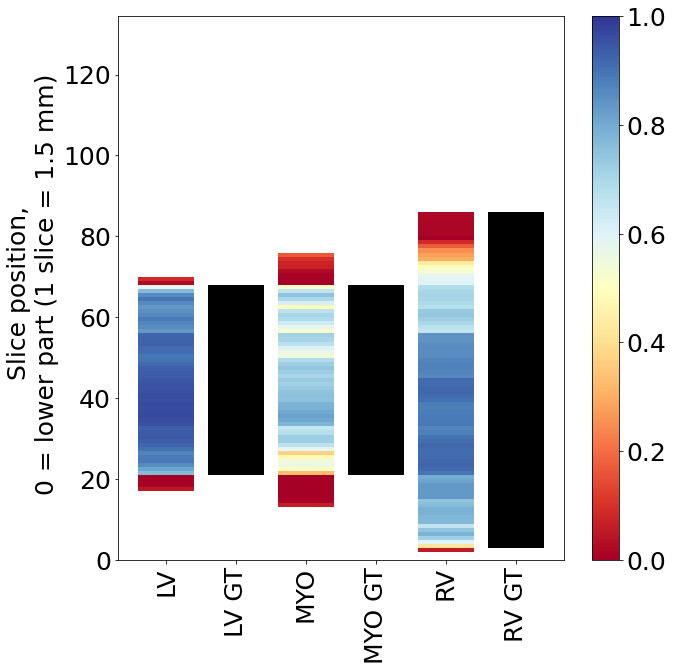}
  \captionof{figure}{Chart for a randomly picked AX sample result of the full pipeline. The x-axis shows one bar per predicted label (LV, MYO and RV). The y-axis indicates the position of the slice in the volume, starting at the lowest slice. 2D Dice is color coded per slice. The black bars show over which slices the respective ground truth (GT) label spans along $z$. 
   Other random examples showed a very similar picture. It seems that our approach slightly over-segmented the LV and MYO, whereas the RV was under-segmented compared to the AX ground truth masks.}
  \label{fig:error_per_labelandslice}
\end{minipage}
\end{figure}

\begin{figure}[t]
    \centering
    \includegraphics[width=1\linewidth]{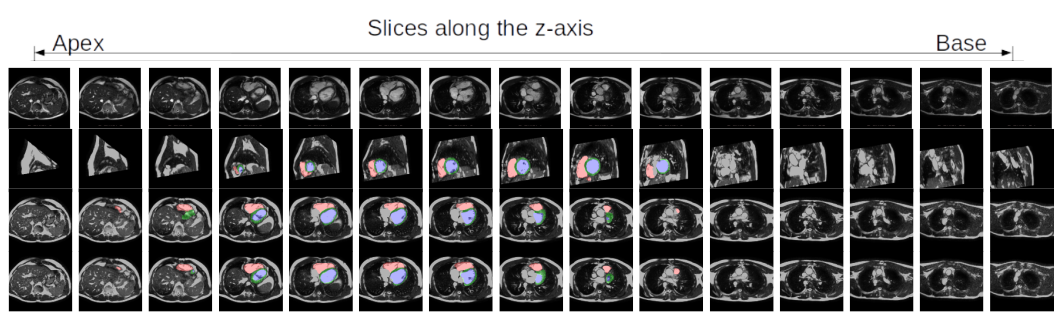}
    \\
    \includegraphics[width=1\linewidth]{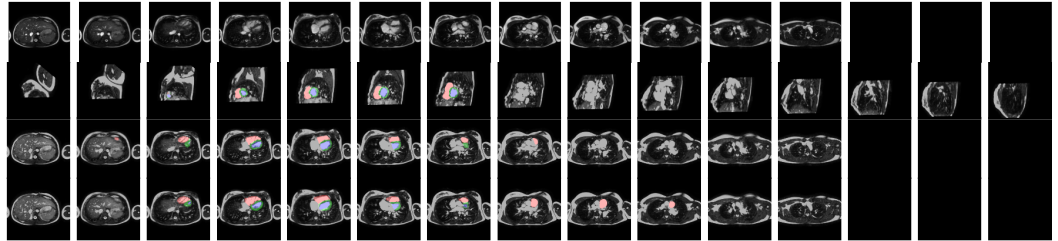}
    \\
    \includegraphics[width=1\linewidth]{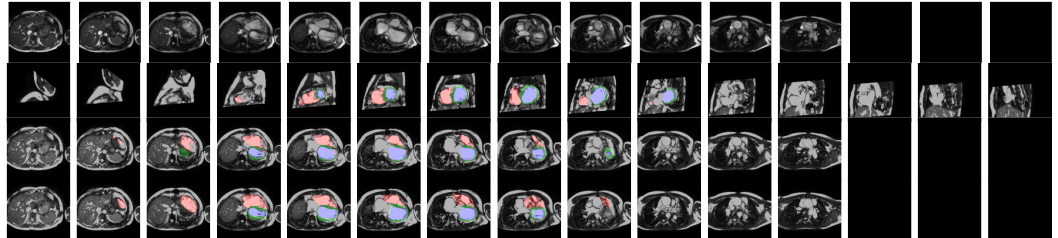}
    \\
    \includegraphics[width=1\linewidth]{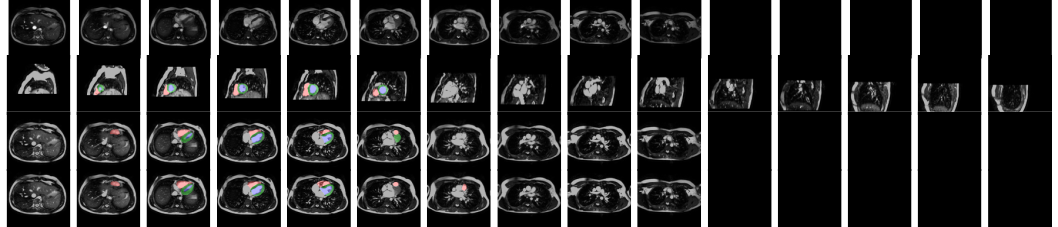}
    \\
    \includegraphics[width=1\linewidth]{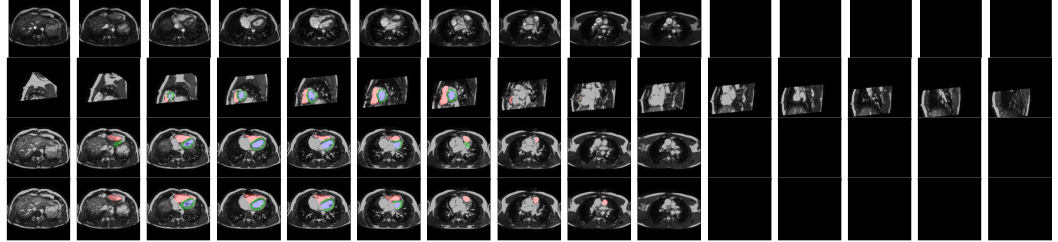}

    \caption{\label{fig:further_ax2sax_transformations} Five example predictions of the final pipeline on the isotropic resampled AX (first row) input CMR. Second row: AX CMR image transformed into the SAX domain and the overlaid predictions of the injected segmentation module; third row: Input AX CMR stack overlaid by the inverse transformed predicted mask; Fourth row: Input AX CMR stack overlaid by the ground truth AX mask. Four rows belong to the same case. The plots show every 8th $z$-slice of the volume.}
\end{figure}

\begin{algorithm}
\SetAlgoLined
\KwResult{One trained transformation model per fold.}
\SetKwInOut{Input}{Input}\SetKwInOut{Output}{Output}
\Input{Hyperparameters}
\Output{Network weights and the following output images: 
$I_{m}, M, I_{t}, M_{t}, J_{m}, Q_t, Q_{tt}$}

\For{fold in folds}
{
 \For{epoch in epochs}
    {
    \For{batch in fold}
        {
        \tcp{Load and pre-process one batch, for simplicity we assume  batchsize=1 }
        \tcp{$\hat{I}=\mathcal{T}(I, \hat{R}\hat{T})$, $\hat{J}=\mathcal{T}(J, \hat{R}\hat{T})$}
        $I,J,\hat{I},\hat{J} \leftarrow load\_and\_preprocess(batch)$\;

        \tcp{Forward the axial image $I$ through the Localisation net $f_{\textrm{loc}}$}
        
        $\phi, \theta, \psi, \vec{t}, \vec{t_{t}}  \leftarrow f_{\textrm{loc}}(I)$\;
        with:  $\vec{t} = [t_{x}, t_{y}, t_{z}]^{T}, \vec{t_{t}} = [t_{xt}, t_{yt}, t_{zt}]^{T}$\;
        
        \tcp{Combine the rotation and translation parameters within the Euler2Affine layer $f_\textrm{e2a}$, $M=RT$}
        $M, M^{-1} \leftarrow f_\textrm{e2a}(\phi, \theta, \psi, \vec{t})$\;
        $M_{t}, M_t^{-1} \leftarrow f_\textrm{e2a}(\phi, \theta, \psi, \vec{t_{t}})$\;

        \tcp{Apply transform operation $\mathcal{T}$}
        $I_{m} \leftarrow \mathcal{T}(I,M)$\;
        $I_{t} \leftarrow \mathcal{T}(I,M_{t})$\;
        $J_{m} \leftarrow \mathcal{T}(J,M^{-1})$\;
        
        \tcp{Apply the pre-trained task module $f_\textrm{task}$ slice-based and use output in $Loss_{focus}$}
        $Q_t \leftarrow f_\textrm{task}(I_t)$\;
        \tcp{For computation of performance metric in target domain:}
        $Q_{tt} \leftarrow \mathcal{T}(Q,M_t^{-1})$\;
        
        \tcp{Calculate the losses}
        $Loss_{cycle} \leftarrow $ Eqn. (13)\;
        $Loss_{focus} \leftarrow $ Eqn. (14)\;
        
        }
    }
    $apply\_gradients\_with\_optimizer([Loss])$\;
    $shuffle(fold)$\;
 }
 \caption{Training one Experiment}
\end{algorithm}
